# Supplementary material for: Optimizing Speech Recognition For The Edge
Source: arXiv:1909.12408 source file (2020-02-07)
Supplement: Supplementary file 1 [file Appendix.tex]

\subsection{Model WER vs Model Size}
See Figure~\ref{fig:WERSizeTradeoff}.
\begin{figure*}[h!]
  \centering
  \includegraphics[width=\textwidth]{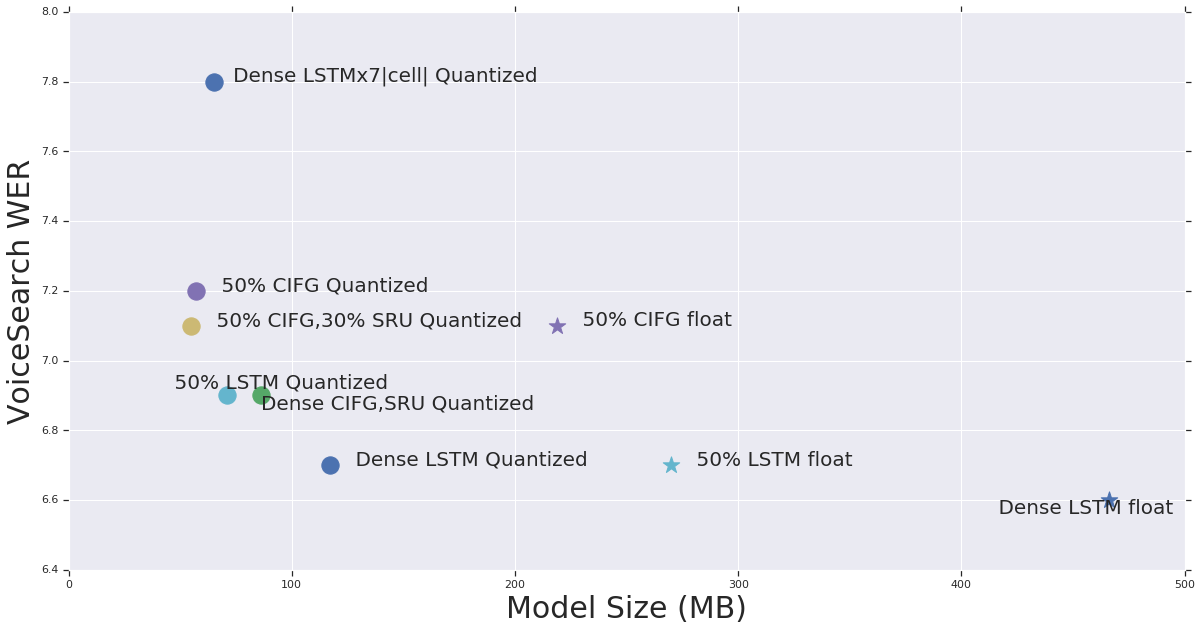}
  \caption{Voice Search WER vs. Model Size (MB).}
  \label{fig:WERSizeTradeoff}
\end{figure*}

\subsection{CIFG vs LSTM experiments}
See Table~\ref{tab:Appendixtab1}.

\begin{table*}[h!]
\centering
\begin{tabular}{|l|l|l|l|c|l|l|} \hline  %YouTube here is YT_VOD17 updated on 5th Sept
                        & Enc \& Dec Cell         & Sparsity  & \#Params (millions) & \multicolumn{3}{c|}{WER} \\\hline
                        & $\times$\#layers        &           & \% of baseline      & VoiceSearch  & YouTube  & Telephony    \\\hline
LSTM                    & LSTMx8                  & -         & 122.1       & 6.6          & 19.5     & 8.1          \\
(Baseline)              & LSTMx2                  & -         & (100\%)     &              &          &              \\\hline
LSTM                    & LSTMx8: $0.7\times|cell|$ & -       & 67.7        & 7.8          & 20.3     & 8.6            \\
(Baseline small)        & LSTMx2: $0.7\times|cell|$ & -       & (55.4\%)    &              &          &                \\\hline
CIFG                    & CIFG-LSTMx8             & -         & 95.8        & 6.8          & 18.6     & 8.1          \\   %SODACifgNoSparse.ckpt-00311460
                        & CIFG-LSTMx2             & -         & (79\%)      &              &          &              \\\hline
Sparse LSTM             & LSTMx8                  & 50\%      & 69.7        & 6.7          & 20.3     & 8.2          \\   % PruningModel.07.30.qo.ckpt-00177540
                        & LSTMx2                  & 50\%      & (57\%)      &              &          &              \\\hline
Sparse CIFG             & CIFG-LSTMx8             & 50\%      & 56.3        & 6.9          & 21.0     & 8.1          \\   % SODACifg50SparseGradualPostTrain.ckpt-00292200
                        & CIFG-LSTMx2             & 50\%      & (46\%)      &              &          &              \\\hline
\end{tabular}
\caption{Comparison of LSTM based RNN-T model with CIFG-LSTM based RNN-T models.}\label{tab:Appendixtab1}
\end{table*}

\subsection{SRU Experiments}
See Table~\ref{tab:Appendixtab2}.

\begin{table*}[h!]
\centering
\begin{tabular}{|l|l|l|c|l|l|l|}\hline % updated YT on 5th Sept
                        & Enc \& Dec Cell       & \#Params (Mil) &\multicolumn{3}{c|}{WER}            \\\hline
                        & $\times$\#layers      & \% of baseline      & VoiceSearch  & YouTube   & Telephony \\\hline
LSTM                    & LSTMx8                & 122.1 (100\%)       & 6.6          &  19.5     & 8.1      \\
(Baseline)              & LSTMx2                &                     &              &           &          \\\hline
SRU-dec                 & LSTMx8                & 111.6 (91\%)        & 6.7          &  18.5     & 8.1      \\   %SODASRUDecOnly.ckpt-00342460
                        & SRUx2                 &                     &              &           &          \\\hline
SRU-dec deep            & LSTMx8                & 124.7 (102\%)       & 6.5          &  18.2     & 7.7      \\   %SODASRUDecDeep.ckpt-00312220
                        & SRUx4                 &                     &              &           &          \\\hline
SRU-enc0                & SRUx2,LSTMx6          & 111.6 (91\%)        & 7.0          &  20.6     & 8.4      \\   %SODASRUEnc0LSTMEnc1LSTMDec.ckpt-00286340
                        & LSTMx2                &                     &              &           &          \\\hline
SRU-enc1                & LSTMx2,SRUx6          & 90.6 (74\%)         & 7.2          &  19.0     & 8.5      \\   %SODALSTMEnc0SRUEnc1LSTMDec.ckpt-00301200
                        & LSTMx2                &                     &              &           &          \\\hline
SRU (long lr)           & SRUx8                 & 69.6 (57\%)         & 8.6          &  21.2     & 10.0     \\   %SODASRUNoSparseCont.ckpt-00313760
                        & SRUx2                 &                     &              &           &          \\\hline
\end{tabular}
\caption{Comparison of RNN-T models that contain SRU cells in the encoder0,
encoder1, and/or decoder. The `long lr' stands for double the learning rate
schedule.}\label{tab:Appendixtab2}
\end{table*}

A LSTM cell contains roughly two times the number of parameters as a SRU cell.
To keep the decoder parameter count unchanged, we stacked 4 layers of SRU cells as the decoder.
Compared to LSTM based decoder, 4 layer SRU improved VoiceSearch, YouTube, and Telephony
test sets by 1.5\%, 6.7\% and 4.9\% respectively.

We also experimented with mixing SRU layers and LSTM layers in the encoder.
Although the resultant models had better WER than the model using SRU layers alone,
they are still not on par with LSTM based encoder. Last but not least, we found
SRU layers needing more time to converge than LSTM layers.
We lengthened the warm-up period, peak period and
decay learning rate schedule by $2\times$, and observed
a 8.5\% drop in the VoiceSearch test set WER of SRU-based RNN-T from 9.4\% to
8.6\%. Similar LSTM based cells could achieve that result with half the learning rate schedule.
